# Supplementary material for: Towards Deployment-Efficient Reinforcement Learning: Lower Bound and Optimality
Source: arXiv:2202.06450 source file (2022-08-31)
Supplement: Supplementary file 1 [file Appendix_AlternativeProof_LB4ArbitraryPolicy.tex]

\section{Alternative Proof for the Lower Bounds}
\subsection{Basic Intuition}
We use $F^{k,kh}_{\psi}$ to denote the event that in the first $k$ deployments, there is no data hit core state at $kh$ (or say, we do not observe non-absorb states in layer $kh+1$ in all previous trajectory), and use $P_{\psi}(F^{k, kh}_{\psi})$ to denote its probability. Then we have,
\begin{align*}
    P_{\psi}(F^{k, kh}_{\psi}) \geq& P_{\psi}(F^{k, kh}_\psi, F^{k-1,(k-1)h}_M) = P_{\psi}(F^{k, kh}_\psi|F^{k-1,(k-1)h}_{\psi}) P_{\psi}(F^{k-1,(k-1)h}_{\psi})\\
    \geq& ...\\
    \geq&P_{\psi}(F^{1, h}_\psi) \prod_{k'=2}^k P_{\psi}(F^{k', k'h}_\psi|F^{k'-1,(k'-1)h}_{\psi}) 
\end{align*}
Next, we try to provide a lower bound for $P_{\psi}(F^{k, kh}_\psi|F^{k-1,(k-1)h}_{\psi})$. An easy fact is that:
\begin{align*}
    P_{\psi}(F^{k, kh}_\psi|F^{k-1,(k-1)h}_{\psi}) =& \sum_{M \in \cM} P_{\psi}(F^{k, kh}_\psi|F^{k-1,(k-1)h}_{\psi}, M) P_{\psi}(M|F^{k-1,(k-1)h}_{\psi}) \\
    =& \sum_{\tau\in F^{k-1,(k-1)h}_{\psi}} p(\tau\in F^{k-1,(k-1)h}_{\psi})\sum_{M \in \cM} P_{\psi}(F^{k, kh}_\psi|\tau, M) P_{\psi}(M|\tau) \\
    \geq& \sum_{\tau\in (F^{k-1,(k-1)h}_{\psi}- Incompelte)} p(\tau\in F^{k-1,(k-1)h}_{\psi})\sum_{M \in \cM} P_{\psi}(F^{k, kh}_\psi|\tau, M) P_{\psi}(M|\tau)
\end{align*}
Given a trajectory $\tau$, we use $h_\tau$ to denote the layer such that there is no non-absorb states in layer $h_\tau+1$ occurs in $\tau$ but we can observe non-absorb states in layer $h_\tau$, or equivalently, the core state at layer $h_\tau-1$ has been hit in $\tau$ while no trajectory in $\tau$ hit core state in $h_\tau$. Then, we can compute that:
\begin{align*}
    P_\psi(M|\tau)=\frac{P_0(M)P_\psi(\tau|M)}{\sum_{M\in\cM}P_0(M)P_\psi(\tau|M)} = \frac{1}{|\cM_\tau|},\quad\forall M \in \cM_\tau
\end{align*}
where we use $\cM_\tau$ to denote the MDPs whose core states in previous $h_\tau$ layers are the same as reflected in $\tau$ while the core states and optimal states in layers starting from $h_\tau+1$ can varies.

Moreover, we can lower bound the average failure rate:
\begin{align*}
    \frac{1}{|\cM_\tau|}\sum_{M\in \cM_\tau} P_\psi(F_\psi^{k,kh}|\tau, M)=\sum_{M\in \cM_\tau} P_\psi(F_\psi^{k,kh}|\tau, M)P_\psi(M|\tau) \geq 1-\frac{N}{d^{2h-h_\tau}} \geq 1-\frac{N}{d^h}
\end{align*}
we would like to choose $h = \log_d NH = \Theta(\log_d H)$ such that,
\begin{align*}
    P_\psi(F_\psi^{k,kh}|\tau, M) \geq 1-\frac{N}{d^h} \geq 1-1/H
\end{align*}
As a result,
\begin{align*}
    P_{\psi}(F^{k, kh}_\psi|F^{k-1,(k-1)h}_{\psi}) =& \sum_{\tau\in F^{k-1,(k-1)h}_{\psi}} p(\tau\in F^{k-1,(k-1)h}_{\psi})\sum_{M \in \cM} P_{\psi}(F^{k, kh}_\psi|\tau, M) P_{\psi}(M|\tau) \\
    \geq& \sum_{\tau\in F^{k-1,(k-1)h}_{\psi}} p(\tau\in F^{k-1,(k-1)h}_{\psi})\sum_{M \in \cM} P_{\psi}(F^{k, kh}_\psi|\tau, M) P_{\psi}(M|\tau)
\end{align*}
As a result, for arbitrary $k\leq K \leq H/\log_d H$, we have:
\begin{align*}
    P_\psi(F_\psi^{k,kh}) \geq (1-\frac{1}{H})^k \geq  (1-\frac{1}{H})^H \geq \frac{1}{e}
\end{align*}

$$
P_\psi(\tau) = \sum_{M\in \cM} P_0(M)P_\psi(\tau|M)
$$
